# Supplementary material for: On the Evaluation of Procedural Level Generation Systems
Source: arXiv:2404.18657 source file (2024-04-29)
Supplement: Supplementary file 1 [file appendix.tex]

\section{Feature Key}

\textbf{Initial Filter}
\begin{enumerate}
\item Paper Accessible: IF1
\item Introduces novel system: IF2
\item Includes Evaluation: IF3
\end{enumerate}
\textbf{Comparison Point}
\begin{enumerate}
\item With Algorithm vs Without: C1
\item Alternative Parameterisation: C2
\item Alternative Algorithms: C3
\item System from Prior Research: C4
\item Multiple Alternative Generators: C5
\item Exemplar Content: C6
\end{enumerate}
\textbf{Method of Evaluation}
\begin{enumerate}
\item Representation Directly: M1
\item Play or Observed Play by Humans: M2
\item Agent Simulation: M3
\item Evaluated through Designing a Level: M4
\end{enumerate}
\textbf{Features Extracted}
\begin{enumerate}
\item Fitness: F1
\item Playability/Win Rate: F2
\item Validated Questionnaire: F3
\item Custom Questions: F4
\item Biological Readings: F5
\item Computational Resource: F6
\item Qualitative Visual Traits of a Sample: F7
\item Metric Diversity: F8
\item Similarity to training levels: F9
\item ERA: F10
\item Controllability: F11
\item Performance as Agent Curriculum: F12
\end{enumerate}
\textbf{Game Domain}
\begin{enumerate}	
\item Mario AI Benchmark: G1
\item GVGAI: G2
\item Commercial Game or Commercial Game Mod: G3
\item Custom System Just for Paper: G4
\item Pre-Existing Research Platform or Framework: G5
\end{enumerate}

\section{Papers Surveyed}

\clearpage
\begin{landscape}
\begin{table}
\tiny
\centering
% [inline block 0: 1 envs, 100032 chars -> data_tex | \begin{tabular}{|p{1cm}|p{1cm}|p{0.28cm}|p{0.20cm}|p{0.20cm}|p{0.20cm}|p{0.20cm}|p{0.20cm}|p{0.20cm}|p{0.20cm}|p{0.20cm}...]

\end{table}

\end{landscape}
